# Supplementary material for: Indiscriminate Data Poisoning Attacks on Pre-trained Feature Extractors
Source: arXiv:2402.12626 source file (2024-02-20)
Supplement: Supplementary file 1 [file appendixs.tex]

\section{Input space attacks}

To begin with our series of experiments, we try out existing attacks such as GC and TGDA without any constraints on the poisoned data.
\red{TO DO: Run GC and TGDA experiments}

We can see that GC in particular works very well when it is added without any constraints. However, when we add in the min-max bounded constraint, neither of the attacks lead to any significant accuracy drop.
\red{TO DO: Run GC and TGDA experiments with constraints}

This suggests that a big reason that GC and TGDA may have worked well was having large values that go way beyond the min-max bound.
Indeed, GC and TGDA generated poisons that are magnitudes greater than the original $[0, 1]$ bound of each pixel in the CIFAR-10 dataset. 
\red{Show metric here}

Given this hypothesis, we tested that even if we take our poisoned data as large random noise, we are able to induce large accuracy drops (as shown in table II and IV). The reason that injecting large random noise works is that large random noise also leads to large points in the feature space \red{double-check this}. Having large points in the feature space then leads to excessively large gradient steps that makes the algorithm impossible to converge. \red{Show gradients and math?}

\blue{Mention something about random points attack vs. model complexity here?}

\red{Note:} In the fine-tuning case, we cannot include the argument about batch norm because it doesn't do anything to batch norm.

\red{We may not want to include the following paragraphs, because they are done with respect to end-to-end training, not fine-tuning.}

Given this hypothesis, we tested that even if we take our poisoned data as large random noise, we are able to induce large accuracy drops. In fact, a single point large enough can cause catastrophic damage to the model even if we allow end-to-end training, as shown in table \ref{tab:single-large}.

\begin{table*}[ht]
    \centering
    %\small
    \caption{Single large data point attack CIFAR-10 with resnet-18}
    \label{tab:single-large}    
    %\scriptsize
    \setlength\tabcolsep{6pt}
   \begin{tabular}{lcccccccccc}
\toprule
\bf $\alpha$ & clean & 0 & 1 & 2 & 3 & 4 & 5 & 6 & 7 \\

\midrule

 & 73.33\% & 68.54\% & 11.28\% & 10\% & 10\% & 10\% & 10\% & 10\% & 10\%   \\

\bottomrule
\end{tabular}
\end{table*}

The reason that such an attack works is because it magnifies the batch norm's running average in Resnet-18.
In table \ref{tab:batch-norm-mean}, we can see that the first batch norm layer has a abnormally large mean due to learning on the single large data point.
After the first batch norm layer normalizes the large data point, mean and variance of subsequent batch norm layers become much smaller, in the same magnitude of clean training. 
When classifying points between $[0, 1]$, the first batch norm normalizes data with its magnified mean and variance and lose meaning. 
\begin{table*}[ht]
    \centering
    %\small
    \caption{l2 norm of running (mean, variance) for various batch norm layers on CIFAR-10 resnet-18 after epoch 1}
    \label{tab:batch-norm-mean}    
    %\scriptsize
    \setlength\tabcolsep{6pt}
   \begin{tabular}{lcccccccccc}
\toprule
\bf $\alpha$ &
 clean & 0 & 1 & 2 & 3  \\

\midrule

First batch norm & 0.33 , 1.03 & 0.29 , 1.18 & 19.57 , 7.16 & 174.2 , 662.15 & 1753.34 , 57153.35   \\
Second batch norm & 5.72 , 13.49 & 5.45 , 10.79 & 3.85 , 9.68 & 3.64 , 9.6 & 4.97 , 10.15   \\
Third batch norm & 4.96 , 9.98  & 4.79 , 10.78 & 4.03 , 9.63 & 5.09 , 9.2 & 4.4 , 8.8  \\
Last batch norm & 10.58 , 16.02  & 11.25 , 16.12 & 10.45 , 15.4 & 12.47 , 16.2 & 11.12 , 15.29   \\

\bottomrule
\end{tabular}
\end{table*}

\section{Fine-tuning}

\textbf{Threat Model:} We first perform experiments on contrastive learning methods on the CIFAR-10 dataset. We apply ResNet-18 as the encoder and choose the feature representation learned by SimCLR with a feature dimension equal to 512. By performing fine-tuning on only the final linear layer (e.g., linear evaluation), the clean accuracy is 84.98\%.

\subsection{Input space attack}
Here we study injecting poisoned data from the input space, which affects the representation indirectly.

\textbf{The simplest attack:} 
Without considering a data sanitization defense, we propose the simplest attack, which simply injects poisoned points with random values. Here we assign $\epsilon_d |\Dtr|$ poisoned points to be $X_p = r * 10^{\alpha}$, where $r$ is a tensor with a random value in the range of $[0,1]$, and $\alpha$ measures the magnitude of poisoned samples. 

\begin{itemize}
    \item \textbf{Different heads}: Here we study the effect of $\alpha$ on different head models in Table \ref{tab:random}.

\begin{table*}[ht]
    \centering
    %\small
    \caption{Random points attack with different $\alpha$. Here we fine-tune the model for 50 epochs. }
    \label{tab:random}    
    %\scriptsize
    \setlength\tabcolsep{6pt}
   \begin{tabular}{lcccccccc}
\toprule
\bf $\alpha$ &
 clean & 0 & 1 & 2 & 3 & 4 & 5  \\

\midrule

FC &  84.98\% & 83.82\% & 80.83\% & 16.53\% & 10.00\% & 10.00\% & 10.00\%   \\

2-Layers & 85.10\% & \bf 84.46\% & \bf 82.89\% & \bf 31.70\% &  10.00\% &  10.00\% &  10.00\%   \\

3-Layers & 84.99\% & 83.49\% & 79.03\% & 22.08\% & 10.00\% & 10.00\% & 10.00\% \\

4-Layers & 10.00\%  &10.00\% &10.00\% &10.00\% &10.00\% &10.00\% &10.00\% \\

\bottomrule
\end{tabular}
\end{table*}

We observe that with a fixed feature representation, (1) all head models degrade to random guess after injecting poisoned points with $\alpha \geq 3$; (2) increasing the complexity of the head model is not always beneficial, e.g., fine-tuning 4-Layers MLP always leads to random guess, even for clean training points; (3) 2-Layer MLP appears to more robust against the simplest attack, especially when $\alpha=2$.

\item \textbf{Different unfreezing layers}: Here we gradually unfreeze the convolutional layers before the linear layer and perform fine-tuning again. We report our results on ResNet 18 in Table \ref{tab:unfreeze} for gradually varying the unfreezing layers from one FC layer to the entire network. Here we observe: (1) Surprisingly, unfreezing more layers for fine-tuning on the clean data is not always optimal: where the accuracy generally drops for unfreezing more blocks, especially when we enter a new block and might sabotage the residual connections; (2) However, we find that fine-tuning more layers (restricted to block 5 and block 6) significantly improves the robustness of the model against the large magnitude attack, especially for $\alpha=2,3$; (3) This suggests that without a proper data sanitization defense, a simple defense strategy against outliers with large magnitude is to fine-tune more (but limited number of) layers.

\begin{table*}[ht]
    \centering
    %\small
    \caption{Random points attack with different $\alpha$ for unfreezing layers starting from the bottom of the architecture to the top. Here we fine-tune the model for 50 epochs.  Here we mark BatchNorm (BN) layers in \vio{violet}, Conv2d (CNN) layers in \teal{teal}, and downsample (DS) layers in \blue{blue}. }
    \label{tab:unfreeze}    
    %\scriptsize
    \setlength\tabcolsep{6pt}
   \begin{tabular}{lcccccccc}
\toprule
\bf $\alpha$ &
 clean & 0 & 1 & 2 & 3  & 4 & 5  \\

\midrule

FC & 84.98\%  & 83.82\% & 80.83\% & 16.53\% & 10.00\% & 10.00\% & 10.00\%   \\
\midrule
+ Linear (9) & 87.33\%  & 87.12\% & 85.15\% & 53.30\% & 10.00\% & 10.00\% & 10.00\%      \\
\midrule
+ \vio{BN} (6.1.2) & 87.33\% & 86.64\% & 85.56\% & 53.85\% & 10.00\% & 10.00\% & 10.00\%   \\

+ \teal{CNN} (6.1.2) & 88.60\% & 88.24\% & 86.06\% &62.11\% &10.00\% &10.00\% &10.00\% \\

+ \vio{BN} (6.1.1) & 88.33\% & 89.14\% & 86.96\% & 68.46\%  & 12.60\% & 10.00\% & 10.00\%  \\

+ \teal{CNN} (6.1.1) & 88.81\% & 89.38\% & 87.91\% & 74.00\% & 15.09\% & 10.00\% & 10.00\%   \\

+ \blue{DS-BN} (6.0.1) & 86.89\% & 88.21\% & 84.01\%  & 68.90\% & 23.87\% & 10.00\% & 10.00\%    \\

+ \blue{DS-CNN} (6.0.0) & 85.77\% & 87.45\% & 86.52\% & 74.15\% & 28.04\% & 10.05\% & 10.00\%\\

+ \vio{BN} (6.0.2) & 89.87\% & 88.06\% & 88.02\% & 76.73\% & 27.82\% & 15.61\% & 10.00\%    \\

+ \teal{CNN} (6.0.2) & 90.12\% & 89.30\% & 88.91\% & 77.71\% & 35.46\% &  15.52\% & 10.00\%  \\

+ \vio{BN} (6.0.1) & 89.08\% & 90.04\% & 87.79\% & 73.24\% & 22.79\% & 10.00\% & 10.00\% \\

+ \teal{CNN} (6.0.1) & 90.19\% & 89.70\% & 88.22\% & 75.10\% & 32.06\% & 10.40\% & 10.00\% \\

\midrule
+ \vio{BN} (5.1.2) & 88.48\% & 86.56\% & 84.89\% & 67.80\% & 14.12\% & 10.00\% & 10.00\%    \\

+ \teal{CNN} (5.1.2) & 89.38\% & 88.68\% & 85.39\% & 70.98\% & 16.37\% & 12.34\% & 10.00\%  \\

+ \vio{BN} (5.1.1) & 86.07\% &  86.91\% & 85.87\% &  76.18\% & 14.67\% & 10.00\% & 10.00\%  \\

+ \teal{CNN} (5.1.1) & 87.38\% & 86.10\% & 86.60\% & 76.10\% & 30.00\% & 10.00\% & 10.00\% \\

+ \blue{DS-BN} (5.0.1) & 86.36\% & 86.38\% & 79.52\% & 70.20\% & 32.10\% & 10.00\% & 10.00\%   \\

+ \blue{DS-CNN} (5.0.0) & 86.67\% & 87.89\% & 84.00\% & 69.35\% & 10.00\% & 10.00\% & 10.00\%\\

+ \vio{BN} (5.0.2) & 87.41\% & 88.08\% & 86.82\% & 78.81\% & 39.29\% & 18.46\% & 10.00\% \\

+ \teal{CNN} (5.0.2) & 88.82\% & 86.73\% & 86.13\% & 79.08\% & 52.54\% & 21.75\% & 10.00\%  \\

+ \vio{BN} (5.0.1) & 86.15\% & 86.40\% & 85.67\% & 78.35\% & 52.04\% & 18.76\% & 10.00\% \\

+ \teal{CNN} (5.0.1) & 87.64\% & 88.05\% & 86.07\% & 75.65\% & 63.65\% & 10.00\% & 10.00\% \\

\midrule
+ \vio{BN} (4.1.2) & 82.66\% & 83.05\% & 78.10\% & 63.85\% & 10.00\% & 10.00\% & 10.00\%    \\

+ \teal{CNN} (4.1.2) & 84.56\% & 86.06\% & 84.93\% & 77.66\% & 10.00\% & 10.00\% & 10.00\%   \\

+ \vio{BN} (4.1.1) & 84.21\% & 83.17\% & 84.61\% & 75.70\% & 43.45\% & 17.39\% & 10.00\% \\

+ \teal{CNN} (4.1.1) & 85.72\% & 86.82\% & 84.16\% & 81.05\% & 41.55\% & 30.42\% & 10.00\% \\

+ \blue{DS-BN} (4.0.1) & 84.77\% & 80.79\% & 82.10\% & 63.25\% & 25.49\% & 10.00\%  & 10.00\%  \\

+ \blue{DS-CNN} (4.0.0) & 84.77\% & 86.33\% & 84.85\% & 74.84\% & 17.92\% & 10.34\% & 10.00\% \\

+ \vio{BN} (4.0.2) & 86.90\% & 85.26\% & 83.20\% & 78.32\% & 49.44\% & 10.00\% & 10.00\%\\

+ \teal{CNN} (4.0.2) & 86.88\% & 87.82\% & 85.88\% & 81.15\% & 12.99\% & 10.00\% & 10.00\%  \\

+ \vio{BN} (4.0.1) & 87.68\% & 86.86\% & 86.85\% & 82.79\% & 28.86\% & 10.00\%  & 10.00\%\\

+ \teal{CNN} (4.0.1) & 86.57\% & 85.80\% & 87.22\% & 75.53\% & 28.16\% & 10.00\% & 10.00\%\\

\midrule
+ \vio{BN} (3.1.2) & 83.72\% & 82.64\% & 81.98\% & 49.84\% & 10.00\% & 10.00\% & 10.00\%   \\

+ \teal{CNN} (3.1.2) & 84.66\% & 86.26\% & 82.19\% & 44.99\% & 12.51\% & 10.00\% & 10.00\%    \\

+ \vio{BN} (3.1.1) & 84.28\% & 84.32\% & 83.98\% & 80.92\% & 32.95\% & 10.92\% & 10.00\%  \\

+ \teal{CNN} (3.1.1) & 85.45\% & 85.93\% & 84.72\% & 78.83\% & 58.54\% & 10.22\% & 10.00\% \\

+ \vio{BN} (3.0.2) & 84.79\% & 87.46\% & 84.84\% & 79.98\% & 15.78\% & 10.33\% & 10.00\%  \\

+ \teal{CNN} (3.0.2) & 84.24\% & 84.88\% & 83.31\% & 79.61\% & 10.00\% & 10.00\% & 10.00\%\\

+ \vio{BN} (3.0.1) & 85.83\% & 86.18\% & 82.81\% & 69.45\% & 10.33\% & 10.00\% & 10.00\%\\

+ \teal{CNN} (3.0.1) & 85.26\% & 85.58\% & 84.32\% & 62.70\% & 11.35\% & 10.00\% & 10.00\% \\

\midrule
+ \vio{BN} (1) & 85.41\% & 85.19\% & 84.69\% & 81.41\% & 17.76\% & 10.00\% & 10.00\%\\

+ \teal{CNN} (0) & 81.39\% & 83.25\% & 81.65\% & 79.21\% & 10.02\% & 10.00\% & 10.00\%\\

\bottomrule
\end{tabular}
\end{table*}

\end{itemize}

\textbf{Label flip attack:} random label flip attack is not effective as long as the entire training set $\chi$ is balanced, i.e., there are roughly the same number of samples for each class. However, if we inject clean samples with the same class (falsely labeled), the attack can easily induce a 50\% accuracy drop with $\epsilon_d=0.2$.

\textbf{TGDA attack:} initial results show TGDA is not that effective.

\textbf{GC attack:} Here we first perform GradPC attack with $\epsilon_w=1$, where it induces 49\% test accuracy. Then we run GC to approach the target parameter and achieve 53\% test accuracy. Although effective, there are two drawbacks of GC attack on fine-tuning: (1) The image is not realistic (or similar to training data), in contrast, it just becomes random noise after the first epoch; (2) the poisoned images have relatively large data range, where the maximum magnitude lies near $[800, 1000]$ upon convergence; (3) when we clip the poisoned data back to the legitimate range $[-1,1]$, the attack is not effective anymore, i.e., the accuracy drop is smaller than $\epsilon_d$. In summary, these properties make GC easy to detect and thus might not be realistic. One conjecture is that optimization is harder for finetuning than injecting data from input space.

\subsection{Feature space attack}

From the previous section, we discover that the input space attack, although easy to deploy, only poses an indirect threat to the feature space and is not a valid attack (considering data sanitization defenses) on fine-tuning. In this section, we introduce a much more powerful attack strategy, which directly injects poisoned points into the feature space. 

Given a pre-trained feature extractor $f$, we take the clean distribution $\mu$ and construct the feature dataset $f(\mu)$. In our experiments, $f(\mu)$ is simply a vector for a single datapoint with dimension $d$, where $d=512$ for our contrastive learning experiments. Here we construct the poisoned dataset $\nu^f$ such that the mixed distribution is $\chi=f(\mu)+\nu^f$.

Firstly, we repeat the simple magnitude attack on the feature space, where the clean accuracy is 87.78\%, and $f(\mu) \in [-0.12,0.12]$.
By injecting $\epsilon=3\%$ random points in the range of $[-1,1]$, we acquire the test accuracy of $78.42\%$, with an accuracy drop of $9.36\%$. 
Next, we repeat the GC attack in the above setting. We successfully reduce the test accuracy to 53\% with $\nu^f \in [-0.51,0.51]$. In summary, we find that the feature space attack is much more effective than the input space attack. 

However, the remaining concern lies in the practicality of such attacks, namely that it is not possible to inject features directly into the 
clean dataset. Thus we propose two methods to invert the toxic poisoned features back to the input space:
\begin{itemize}
    \item Autoencoder: Here we first train an autoencoder to reconstruct the training data. However, since the encoder (feature extractor) is fixed, we cannot train the autoencoder end-to-end. In other words, a good feature extractor may not suggest a good encoder. \blue{We successfully trained a U-net with fixed encoders. However, the reconstruction (upsampling) process requires skip connections from the encoder. In practice, we find that these skip connections highly control the reconstructed images.}
    \item PoisonFrog \parencite{ShafahiHNSSDG18}: inspired by the idea of \parencite{ShafahiHNSSDG18}, we propose to learn the poisoned data $\nu^f$ and the feature extractor $f$ with parameter $\theta$. Specifically, we aim at minimizing the following objective function:
    \begin{align}
        \min_{\nu}\mathcal{L} = \min S(\mu,\nu) + \max S(f(\nu),\nu^f)
    \end{align}
\end{itemize}

\begin{table*}[ht]
    \centering
    %\small
    \caption{Comparison between input space attack, U-Net attack, and Feature Targeted attack wrt different $\epsilon_d$.}
    %We set the boundary to be $\epsilon_d=0.2$ as the feature attack returns features with the same range as normal features at this boundary.}
    \label{tab:main}  
    %\scriptsize
    \setlength\tabcolsep{6pt}
   \begin{tabular}{lcccc}
\toprule
\bf Attack & Clean & $\epsilon_d=0.03$ \\

\midrule
Feature & 87.78\% & 53.00\% / -34.78\%  \\

TGDA & 87.78\% & 85.59\% / -2.19\%  \\

GC (with constraints) &  87.78\% & 85.28\% / -2.5\% \\

U-Net & 87.78\% & 83.56\% / -4.22\%    \\

FT ($\beta=0.25$)  & 87.78\% & 82.48\% / -5.3\% \\

FT ($\beta=0.1$) & 87.78\% & 75.34\% / -12.44\%\\

\bottomrule
\end{tabular}
\end{table*}

\noindent \paragraph{Feature attack as target features to data poisoning} Following the above idea of \cite{ShafahiHNSSDG18}, we formally construct the Feature Targeted (FT) attack algorithm.

\begin{algorithm}[t]
\DontPrintSemicolon
    \KwIn{base instances as part of the training distribution $\mu_b = \epsilon_d\mu$,  
    step size $\eta_1$,$\eta_2$, a pre-trained encoder $f$, target features $\nu^f$ (the output of GC feature attack)  }
    
    initialize poisoned dataset $\nu = \mu_b$
    
    \For{$t =1, 2, ...$}{
    Forward step: $\hat{\nu}=\nu - \eta_1\nabla_{\nu}S(f(\nu),\nu^f)$ 

    Backward step: $\nu = (\hat{\nu}+\eta_2\beta\mu_b)/(1+\beta\eta)$
    }

\textbf{return} the final poisoned dataset $\nu$

\caption{Feature Targeted (FT) Attack}
\label{alg:pf}
\end{algorithm}

Following Algorithm \ref{alg:pf}, we choose $\epsilon_d$ and take the target features $\nu^f$ returned by GC, where the test accuracy is 53\% with  $\nu^f \in [-0.51,0.51]$. We observe that:
\begin{itemize}
    \item With only a forward step (no constraints on the input space), we can reduce the loss and achieve the target feature. However, the images quickly converge to random noise, and the magnitude increases to [100,1000]. We clearly see without any constraints, the FT attack returns very similar results with GC in the input space. 
    \item Next we add the forward steps, where the proximal step minimizes the Frobenius distance from the base instances in input space. We observe an accuracy drop of 5.3\% compared to the input space attack (2.5\%) while preserving the magnitude and the realistic feature of $\nu$.
    \item However, there still exists some \textbf{limitations} of the FT attack: (1) The loss converges at a very big number, indicating that the distance still remains large between $\nu$ and $\nu^f$; (2) The accuracy drop is tiny compared to the feature space attack (5.3\% compared with almost 40\%). Both of the findings confirm that the FT attack does not achieve the target feature; (3) To examine the limit of the FT attack, we scale down the magnitude of $\nu^f$ to be the same as $\mu^f$, and observe that the initial loss drops down, but the relative loss decrease stays roughly the same (-10\%), which may indicate that the limit of FT does not only depend on the magnitude of the features; (4) \red{FT attack reachability: why is $\nu^f$ hard to achieve? Is it because the target parameter we choose is too ambitious? Is it because $\epsilon_d$ is too small?}
    \item By varying $\epsilon_d$ and $\epsilon_w$, we observe that the attack is not more effective (even though the features are easier to reach, magnitude-wise), which matches the above findings. This motivates us to further improve the FT attack.
    \item Our current attack selects the target features $\nu^f$ randomly. However, we find that in practice the difficulty of achieving different target features varies significantly, and highly depends on the initial similarity between $f(\nu)$ and $\nu^f$. Thus I propose to have a ranking procedure before the attack for assigning base samples and poison features.  \blue{Updates: The ranking process helps with initialization significantly (we can start from a much lower initial loss) and we can achieve lower convergence loss with less training epochs. } However, this approach does not affect significantly the attack effectiveness, thus we propose another solution.
    \item To make FT attack more effective, we weaken the constraint on the input space (magnitude and whether the samples look realistic) using two approaches: (1) we set different step sizes $\eta_1,\eta_2$ for the forward and backward steps, where $\eta_1>\eta_2$; (2) choose $\beta$ to be smaller. We observe that with weaker constraints, the attack generally becomes more effective, but also involves a tradeoff: the images contain more noise and tend to converge at a larger magnitude (about 7-10 times of the normal magnitude).
\end{itemize}

\red{Plans for next step:}

\begin{itemize}
    \item Verify the Lipschitz constant of the pre-trained model, and check if it is much greater than 1 (if it is, it should be easy to invert the poisoned features back to the input space); \blue{We verify the Lipschitz constant of the pre-trained network using AutoLip and we get about $10^8$ as an upper bound. }
    \item Check the magnitude of perturbation of the feature space attack (e.g., L2 norm), and see if we can add the constraint to the feature space attack: \blue{an effective GC feature space attack incurs perturbation (L2) $\approx 100$ for $\epsilon_d=0.03$, adding constraints on the perturbation would cause GC to be ineffective.  }
    
    \item Revisit the autoencoder architecture and see if it is possible to train an autoencoder without linear layers as a bottleneck. \blue{did not get a good autoencoder yet.}
\end{itemize}

\textbf{Conclusion for fine-tuning tasks:} in this section, we confirm that: (1) fine-tuning pre-trained feature extractors are indeed vulnerable to unbounded indiscriminate data poisoning attacks injected from the input space, e.g., the large magnitude attack and GC attack. However, these attacks become ineffective with explicit constraints, i.e., the visual presentation of the poisoned image and the magnitude of perturbation; (2) treating the pre-trained features as a dataset, we can easily inject poisoned features with (relatively) small perturbations using GC and induce a high accuracy drop. However, the feature space attack is not very realistic; (3) to invert the poisoned features back to the input space, we propose the Feature Targeted (FT) attack. The FT attack is more effective in general, additionally, with explicit constraints, we observe the poisoned points look benign from human eyes.
